# Supplementary material for: Experimental observation of symmetry protected bound state in the continuum in a chain of dielectric disks
Source: arXiv:1806.01932 ancillary file (2018-06-03)
Supplement: Supplementary file 1 [file Supplementary_Information.pdf]

# SUPPLEMENTAL MATERIAL
# Experimental observation of symmetry protected bound state in the continuum in a chain of dielectric disks

M.A. Belyakov[1], M.A. Balezin[1], Z.F. Sadrieva[1], P.V. Kapitanova[1], E.A. Nenasheva[2], A.F. Sadreev[3], A.A. Bogdanov[1]
[1] *Department of Photonics and Metamateials ITMO University St. Petersburg 197101, Russia*
[2] *Giricond Research Institute, Ceramics Co., Ltd., St. Petersburg 194223, Russia*
[3] *Kirensky Institute of Physics Federal Research Center KSC SB RAS 660036 Krasnoyarsk Russia*
(Dated: June 3, 2018)

PACS numbers: 42.25.Fx,41.20.Jb,42.79.Dj

## S1. MATERIAL LOSSES OF CERAMICS

To define the loss tangent of the ceramics, we measured the extinction cross-section of a single ceramic disk [Fig. S1(a)]. To perform the measurements, the ceramic disk was located in the middle between two wideband horn antennas. The antennae were connected to the ports of a vector network analyzer (VNA). The polarization of the incident wave is shown in the inset of Fig. S1(a). The spectrum of the extinction cross-section has been calculated applying the optical theorem. Using the classical Fano formula [1]

$$F(\Omega) = A\frac{(\Omega+q)^2}{\Omega^2+1}, \tag{S1}$$

we extracted the Q-factor of a resonance with the azimuthal number $m = 3$. The distribution of $|\mathbf{E}|^2$ for this resonance is shown in the inset of Fig. S1(a). Here, $\Omega = (\omega-\omega_0)/(\gamma/2)$ is a normalized frequency, $\omega_0$ is the resonance frequency and $\gamma$ is the damping constant of the mode, $q$ is the Fano asymmetry parameter and $A$ is the amplitude of the resonance. The treatment of the experimental data yield the Q factor about $2.3 \times 10^3$. This is the total Q factor, which includes the radiation losses and losses due to absorption in the ceramics:

$$\frac{1}{Q_{\rm tot}} = \frac{1}{Q_{\rm rad}} + \frac{1}{Q_{\rm abs}}. \tag{S2}$$

To find $Q_{\rm abs}$ from Eq. (S2), we obtain the $Q_{\rm rad}$ numerically using Comsol Multiphysycs software. The total Q factor of the analyzed mode equals to $6 \times 10^3$. Substitution of this value to Eq. (S2) gives $Q_{\rm abs} = 4 \times 10^3$.

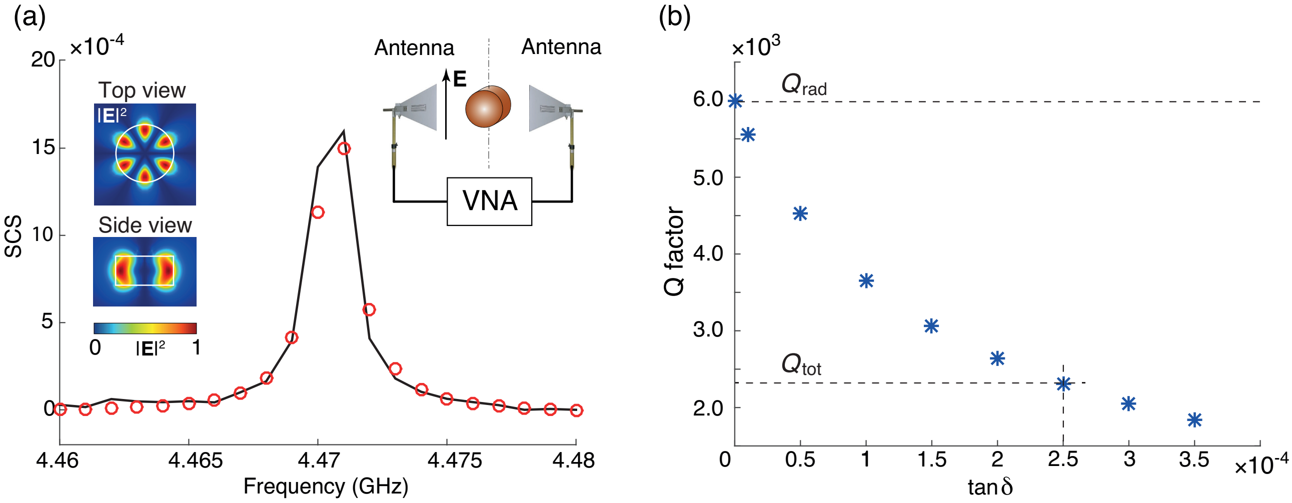


FIG. S1: (a) Measured extinction cross-section of a single ceramic disk. The resonance corresponds to the mode with orbital angular momentum (OAM) $m = 3$. Left inset shows distribution of $|\mathbf{E}|^2$ (top and side view). Right inset shows the scheme of the experiment. The circle markers show the experimental data and the solid line is the approximation. (b) Dependence of the total Q factor for the resonance with $m = 3$ at $\omega_0 = 4.47$ GHz on loss tangent. The dashed lines show

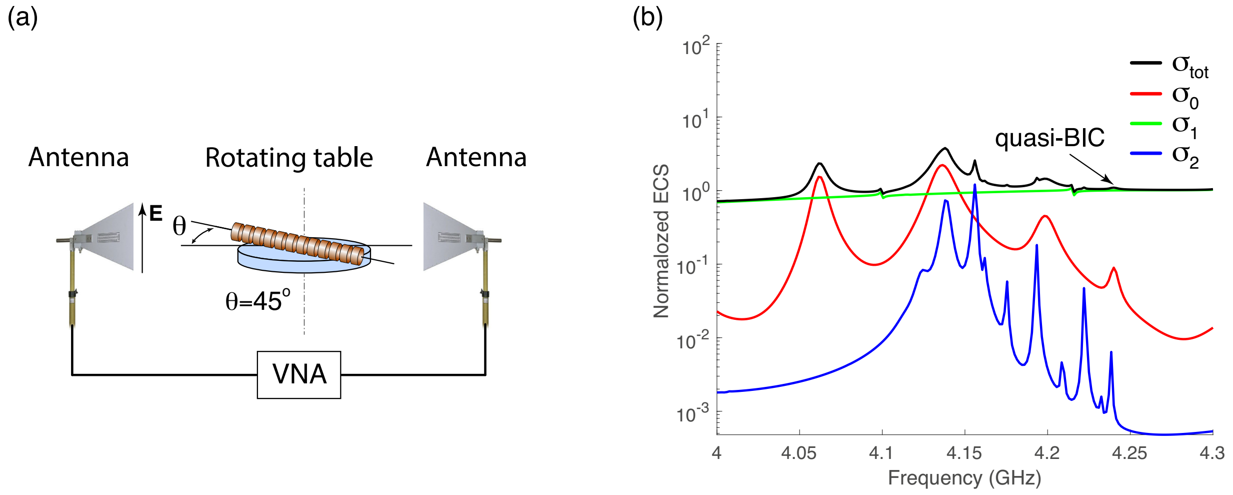


FIG. S2: (a) Scheme of the experiment on measurement of extinction cross-section of the array. (b) Calculated spectra of the total ECS and partial ECSs corresponding to OAM $m = 0, 1, 2$.

According to the definition, the loss tangent $\tan\delta = \varepsilon''/\varepsilon'$, and therefore $\tan\delta = 1/Q_{\rm abs} = 2.5 \times 10^{-4}$. This value corresponds to $\varepsilon'' \approx 0.01$. We also find the dependence of $Q_{\rm tot}$ on $\tan\delta$ numerically using eigensolver of Comsol Multiphysycs [see Fig. S1(b)]. The numerical calculations confirm that $\tan\delta = 2.5 \times 10^{-4}$ gives $Q_{\rm tot} = 6 \times 10^3$ for the resonance at $\omega_0 = 4.47$ GHz. We used the found value of $\tan\delta$ to calculate theoretical dependence of the total Q-factors of the symmetry-protected quasi-BIC on the number of the disks in the array (see Fig. 4 in the main text).

## S2. SCATTERING ON ARRAY OF THE DISCS

A plane wave incident on the array of the chain as demonstrate in Fig. S2(a) excites the modes with all OAM ($m = 0, 1, 2, ...$). For the considered design of the chain (see Fig. 1 in the main text) the transmission band corresponding to $m = 0$ and $m = 2$ overlaps (see Fig. 2(a) in the main text). Therefore, it is difficult to distinguish the resonances corresponding to the modes with $m = 0$ and $m = 2$ in the extinction spectra. Figure S2(b) shows the calculated spectra of partial extinction cross-sections corresponding to $m = 0, 1, 2$ and the total scattering cross-section defined as their sum. It is worth to mention that the modes with $m = 2$ appear in the transmission spectra if the loop antenna placed non coaxially with the chain.

## S3. COUPLING OF DISK ARRAY WITH LOOP ANTENNA

In the general case, the loop antenna used for measurement of the transmission spectra of the disk chain makes an additional contribution into the losses of all resonances, particularly, into the losses of quasi-BIC. To be sure that the additional losses arising due to coupling of the antenna to the array is negligible we provide additional experiments and numerical calculations.

Figure S3(a) shows the experimental transmission coefficient measured for different distances $d$ between the array and antenna. Figure S3(b) shows that there is no dependence of Q factors of the last three resonances of the transmission band on $d$. This confirms indirectly that in the considered range of $d$, the coupling of the array to the antenna is weak and the antenna does not affect the Q factors of the resonances in the main text.

To be sure that we work in the weak coupling regime not decreasing the radiation Q factor of quasi-BIC and other resonances we provide numerical simulation showing the dependence of Q factor on $d$ for a single disk and the array of 20 disks [see Figs. S3(c) and S3(d)]. Our calculations show that the antennas affect the Q factor of the resonances if $d$ is less than about 1.5 mm. In the experiments showed in the main text (see Fig. 3 in the main text).

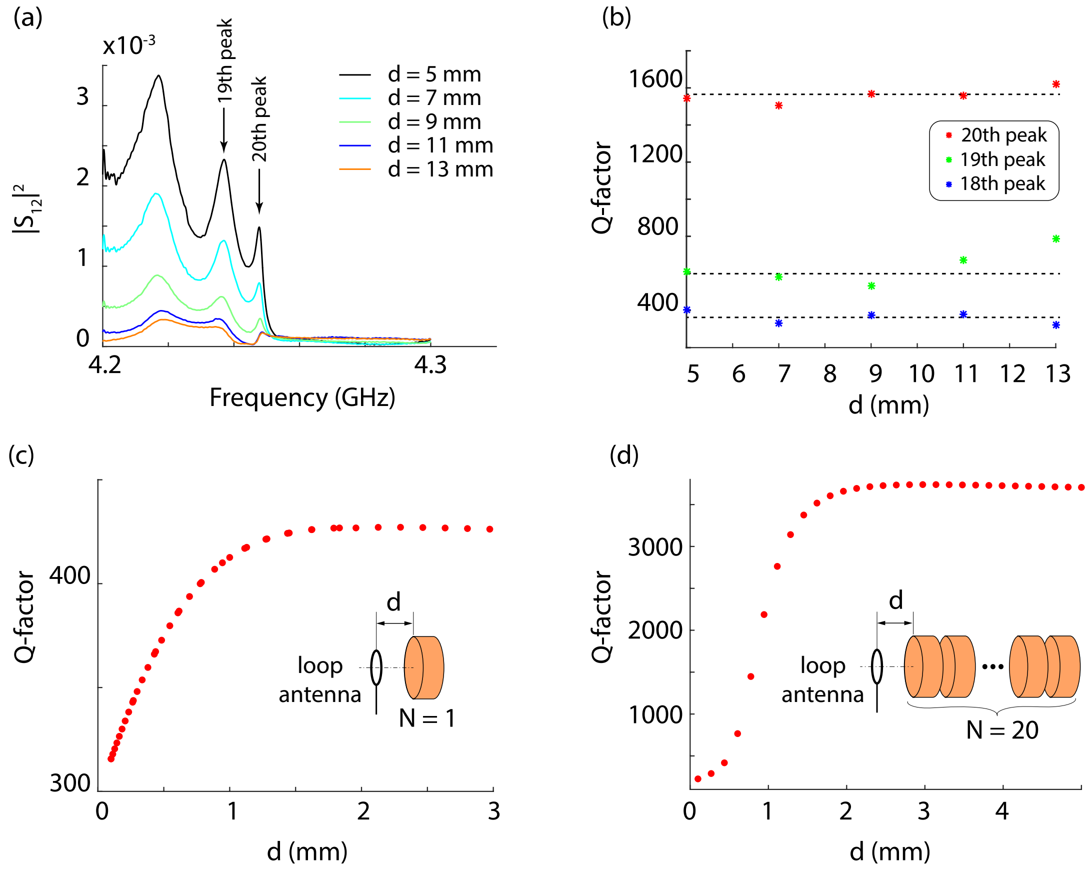


FIG. S3: (a) Transmission spectra $|S_{12}|^2$ of the chain consisting of 20 ceramics disks placed between two coaxially positioned loop antennas measured for different distances $d$ between the antennas and the outermost disks. The parameters of the chain are shown in caption of Fig. 1 of the main text. (b) Measured dependences of the Q factor of the last three resonances of the transmission band depending on the distance $d$ between the antennas and the chain. (c) Numerically calculated dependence of Q factor of the resonance with OAM $m = 2$ at the frequency 3.86 GHz in a single disk on the distance $d$ between the disk and the loop antenna. (d) Numerically calculated dependence of Q factor of the quasi-BIC (20th peak) in chain consisting of 20 disks on the distance $d$ between the outermost disk and the loop antenna. Material absorption in panels (c) and (d) are neglected.

## References


[1] M. V. Rybin, A. B. Khanikaev, M. Inoue, K. B. Samusev, M. J. Steel, G. Yushin, and M. F. Limonov, Phys. Rev. Lett. 103,023901 (2009).
